# Supplementary material for: On the Hardware Feasibility of Nonlinear Trajectory Optimization for Legged Locomotion based on a Simplified Dynamics
Source: arXiv:1910.06855 source file (2020-04-01)
Supplement: Supplementary file 1 [file appendix.tex]

\section{Appendix}
%\subsection{Force polytope's Jacobian}
%One vertex $\vc{f}^{lim}$ of the force polytope $\mathcal{A}_i$ the constraint's Jacobian would require the knowledge of the following quantity:
% \begin{equation}\label{eq:forcePolytopesJacobian}
% \begin{aligned}
% & \frac{d \vc{f}^{lim}(IK(\vc{p}))}{d \vc{p}} = \frac{d \vc{f}^{lim}(\vc{q})}{d \vc{p}} = \frac{d (\vc{J}^{-T}(\vc{q})\vc{\tau}^{lim})}{d \vc{p}}\\
% & = \frac{d \vc{J}^{-T}(\vc{q})}{d \vc{p}}\vc{\tau}^{lim} + \frac{d \vc{\tau}^{lim}}{d \vc{p}}\vc{J}^{-T}(\vc{q})
% \end{aligned}
% \end{equation}
% The above relationship is highly nonlinear because of the trigonometric terms in the leg's Jacobian matrix and it requires the knowledge of the robot's kinematics which is against the \gls{srbd} assumption.
\subsection{Force polytope's Simplified Jacobian}
The simplified force polytope constraint's Jacobian $d \vc{g} / d \vc{x}$ with respect to the optimization variables $\vc{x}$, required by nonlinear optimization solvers based on the interior point method, can be deducted as follows:
\begin{equation}
	\frac{d \vc{g}}{d \vc{x}}  = \frac{d \vc{A}(\vc{p})}{d \vc{x}} \vc{f} + \frac{d \vc{f}}{d \vc{x}} \vc{A}(\vc{p}) - \frac{d \vc{d}(\vc{p})}{d \vc{x}}
\end{equation}
where:
\begin{equation}
	\frac{d \vc{A}(\vc{p})}{d \vc{x}} = \mat{- \sin(\theta_x) \\ \cos(\theta_x)} \cdot \frac{\theta_2 - \theta_1}{p_{2,x} - p_{1,x}} \cdot \frac{d \vc{p}}{d \vc{x}}
	\label{eq:constraintJacobiansA}
\end{equation}
and: 
\begin{equation}
\frac{d \vc{d}(\vc{p})}{d \vc{x}} = \frac{d_2 - d_1}{p_{2,x} - p_{1,x}}
\label{eq:constraintJacobiansD}
\end{equation}
We can see that the above relationship does not depend on the robot's kinematics and it can be therefore applied to arbitrary robots. The three polytopes employed for the morphing are, instead, robot specific and they can be computed offline.
